# Supplementary material for: OPT-GAN: A Broad-Spectrum Global Optimizer for Black-box Problems by Learning Distribution
Source: arXiv:2102.03888 source file (2023-01-31)
Supplement: Supplementary file 3 [file fig_flowchart.tex]

\begin{figure*}
  \centering
  \includegraphics[width=0.8\textwidth]{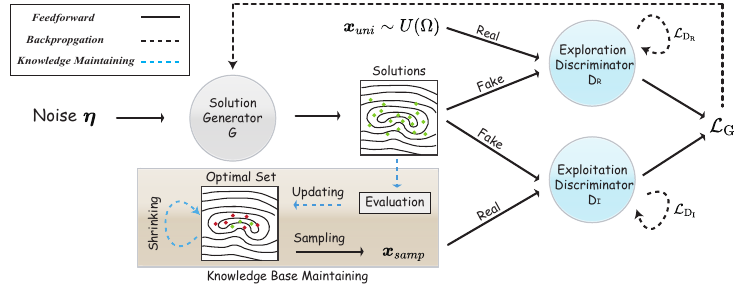}
  \caption{
  Optimization process of the proposed OPT-GAN, which mainly consists of two components: generator pre-training (not drawn in this figure) and distribution reshaping. The generator pre-training initializes the solution generator $G$, and enables it to generate uniformly scattered solutions in the searching domain. In the distribution reshaping, solution generator $G$ generates the solutions of the optimization problem, and is trained according to the loss from $D_{R}$ and $D_{I}$. The optimal set including the historical best solutions is updated by the knowledge base maintaining strategy at each iteration. The best solution in the optimal set is viewed as the optimum when the termination condition is reached.
  } 
  \label{fig:flowchart}
\end{figure*}
